# Supplementary material for: Contact Surface Estimation via Haptic Perception
Source: arXiv:2003.02227 source file (2020-03-04)
Supplement: Supplementary file 1 [file appendix.tex]

\todo{probably won't have any space}

\subsection{Simplified Likelihood function}
\noindent Given a set of observations $\bD$, the observation mean and variance are
\begin{equation}
  \begin{aligned}
  \obsAve &= \frac{1}{n} \sum x_i \\
  \obsVar &= \frac{1}{n-1} \sum_1 ^n ( x_i - \obsAve )^2 
\end{aligned}
\label{e:appendix-observation-variance}
\end{equation}

\noindent The error between observation and the unknown mean 
\begin{equation}
\begin{aligned}
  \sum_i(x_i-\mu)^2 &= \sum \left[ (x_i - \obsAve ) - ( \mu - \obsAve ) \right]^2  \\
		    &= \sum ( x_i- \obsAve )^2 + \sum ( \obsAve - \mu)^2  \\ 
		    &~~~~~~~~~~ - 2 \sum (x_i-\obsAve) (\mu-\obsAve) 
\end{aligned}
\label{e:appendix-observation-minus-mean}
\end{equation}

\noindent From~\eref{appendix-observation-variance}, we know that the first term above can be written as
\[
 \sum (x_i-\obsAve)^2 = (n-1) \obsVar 
\]

\noindent The third term in~\eref{appendix-observation-minus-mean} can be reduced to 0 
\[
\begin{aligned}
 2 \sum (x_i-\obsAve) (\mu-\obsAve) &=2 (\mu-\obsAve) \left[\sum(x_i) - n\obsAve \right]\\
	&= 2 (\mu-\obsAve) \left[ n\obsAve - n\obsAve \right] \\
	&= 0
\end{aligned}
\]

\noindent 
Therefore,~\eref{appendix-observation-minus-mean} can be simplied to 
\begin{equation}
  \sum_i(x_i-\mu)^2 = (n-1) \obsVar + n (\obsAve-\mu) 
\end{equation}

\subsection{Posterior}

\noindent The posterior distribution is the likelihood times the prior

\begin{equation}
\begin{aligned}
\prob{\contactNormal|\bD}
  &=
 \prob{\bD|\contactNormal,\obsPre} \prob{\contactNormal,\obsPre|\mu_0, \kappa_0, \alpha_0,\beta_0}\\
 &= \frac{1}{(2\pi)^{n/2}} \obsPre^{n/2} \exp^{-\frac{\obsPre}{2} \sum ( x_i -\obsAve )^2 } \\
  &\frac{\beta_0^{\alpha_0}} {\varGamma(\alpha_0)}  
  \sqrt{\frac{\kappa_0}{2\pi} } 
  \obsPre^{\alpha_0-0.5} 
  \exp^{ - \frac{\obsPre}{2} \left[\kappa_0 \sum( \contactNormal-\contactNormal_0)^2 + 2\beta_0 \right]}  
\end{aligned}
\end{equation}

\[
 \kappa_0 \sum( \contactNormal-\contactNormal_0)^2 + 2\beta_0 +\sum ( x_i -\obsAve )^2  
\]

\begin{comment}
 
\subsection{Inverse chi-squared distribution}
The scaled inverse chi-squared distribution can be used as a conjugate prior for a normal distribution with unknown variance. 

According to Bayes' theorem, the posterior probability distribution is proportional to the product of the likelihood function and the prior distribution.
\[
 \prob{\sigma^2 | \bD , \bI} \propto \prob{\bD|\sigma^2}\prob{\sigma^2|\bI} 
\]
where $\bD$ denotes the dataset and 
$\bI$ denotes the initial information about $\sigma^2$

The posterior distribution 
 
\subsection{T-distrubtion as conjugate prior}

T-distribution is a probability distribution for estimting the mean of a normally distribution function for small sample size and unknown vairiance.

\end{comment}
